# Supplementary material for: FuRPE: Learning Full-body Reconstruction from Part Experts
Source: arXiv:2212.00731 source file (2024-01-03)
Supplement: Supplementary file 1 [file supp.pdf]

# FuRPE: Learning Full-body Reconstruction from Part Experts

## –Supplementary materials–

Anonymous CVPR submission

Paper ID 5482

### 1. Appendix

This is the supplementary materials of the submitted paper "FuRPE: Learning Full-body Reconstruction from Part Experts". To give the read a better view of understanding our paper, in this document, we add more visualization results. The visualization results include some results on Now dataset for head reconstruction, some results on 3D 3DPW dataset to compare our method with expose, and some failure cases where our methods achieve poor performance on 3DPW dataset. Hope these result can inspire future researches. In Fig. ??, we find that our method can better reconstruct the mouth areas compared to ExPose. Then in Fig. ??, we find our method is obviously better at reconstructing wrists compared to Expose. However, in Fig ??, we can find our method also fails in some cases. For example, when the hands are closed together, our method fails to reconstruct both left and right hands. Future works should make efforts to solve these problems.

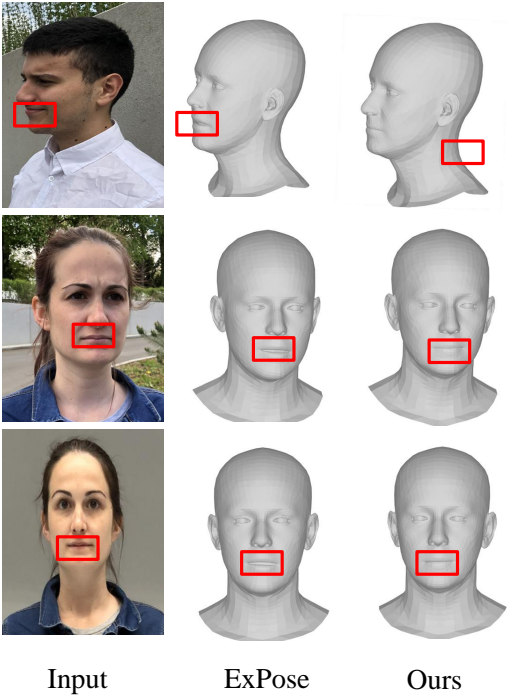

Figure 1. Visualization and comparison on Now dataset.

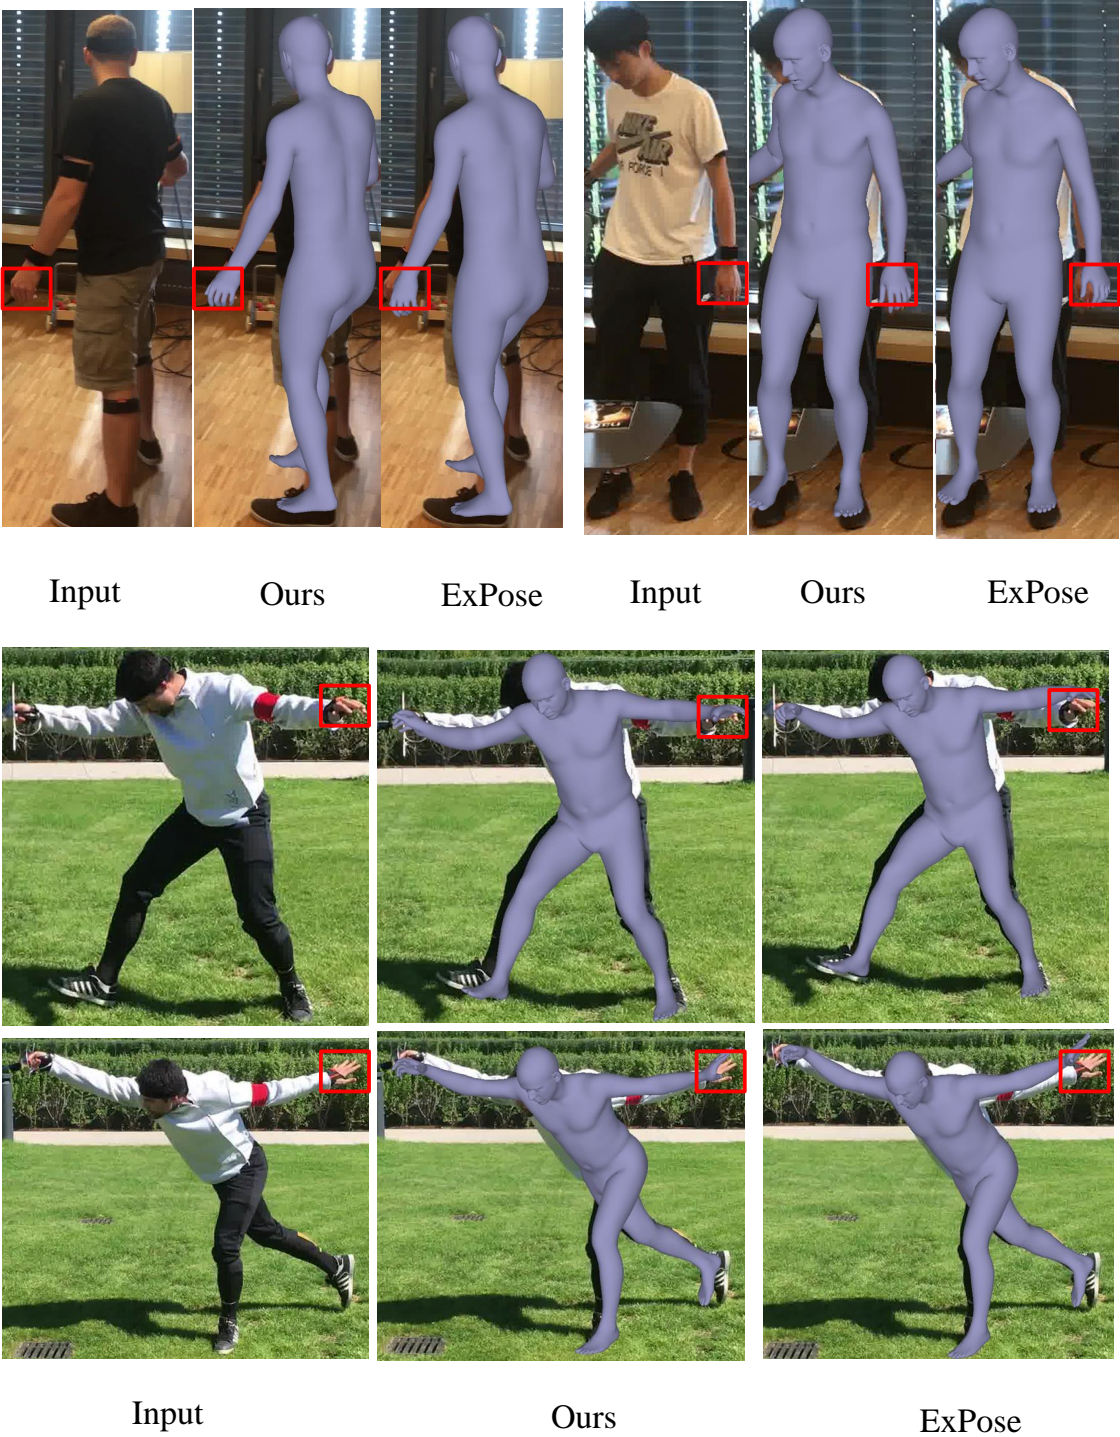

Figure 2. More visualization and comparison on 3DPW dataset.

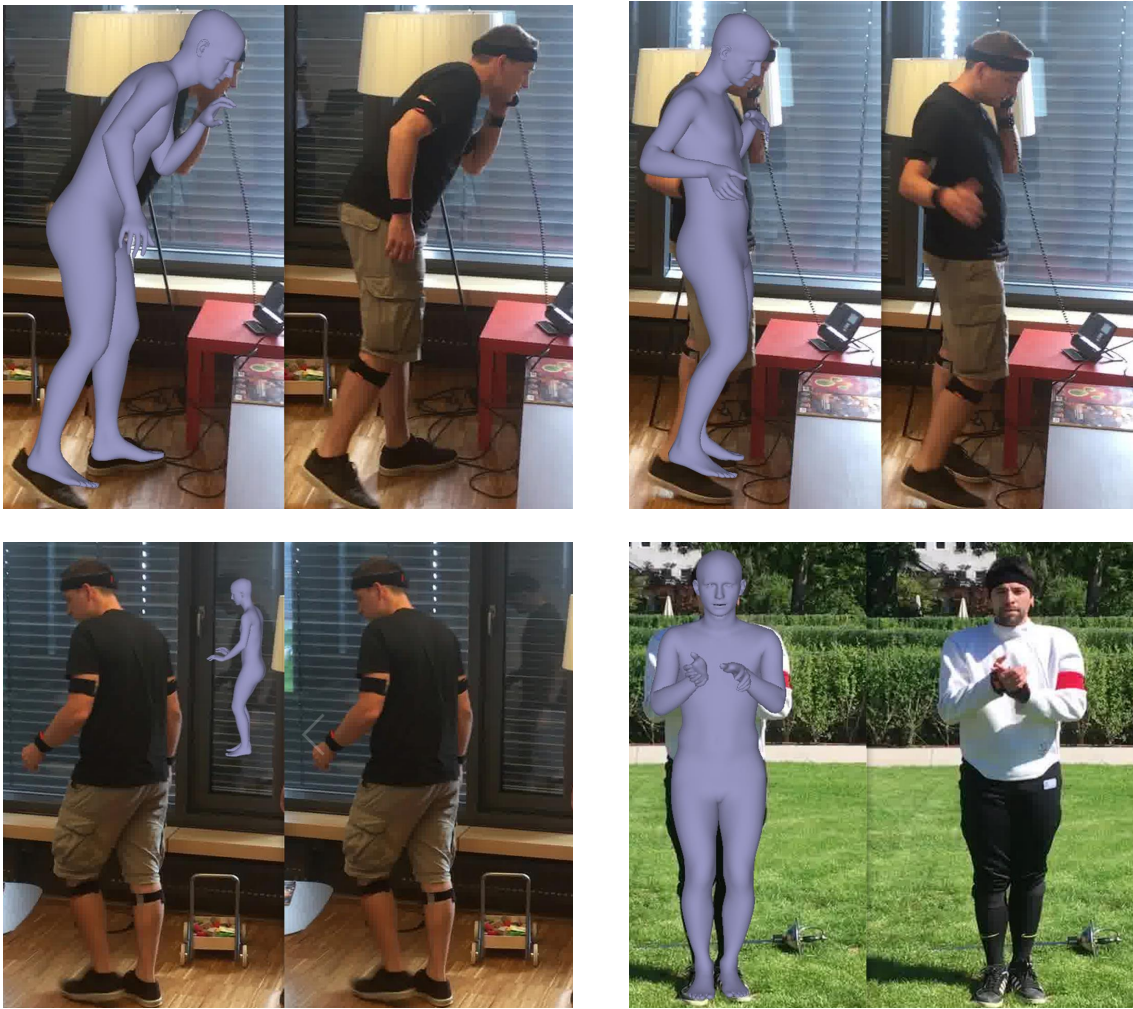

Figure 3. Visualization of some bad cases on 3DPW dataset
